# Supplementary material for: Quantum Monte Carlo study of the energetics of the rutile, anatase, brookite, and columbite TiO$_2$ polymorphs
Source: arXiv:1610.08992 source file (2016-10-27)
Supplement: Supplementary file 1 [file supplementary.pdf]

# Quantum Monte Carlo study of the energetics of rutile, anatase, brookite and columbite $TiO_2$ polymorphs: Supplemental Material

John Trail,[1] Bartomeu Monserrat,[1,2] Pablo López Ríos,[1] Ryo Maezono,[3] and Richard J. Needs[1]

[1]*Theory of Condensed Matter Group, Cavendish Laboratory, J. J. Thomson Avenue, Cambridge CB3 0HE, UK*

[2]*Department of Physics and Astronomy, Rutgers University, Piscataway, New Jersey 08854-8019, USA*

[3]*School of Information Science, JAIST, Asahidai 1-1, Nomi, Ishikawa 923-1292, Japan*

(Dated: October 20, 2016)

Evaluation of total energies for anatase, brookite, columbite, and rutile consist of preliminary density functional theory (DFT) calculations followed by diffusion Monte Carlo (DMC) calculations, with anharmonic vibrational corrections calculated at the DFT level of theory using the vibrational self-consistent field (VSCF) method. In this document we give details of the calculations involved in each of these stages.

## I. DETAILS OF THE DFT CALCULATIONS

For the initial DFT calculations, the correlated-electron pseudopotentials[1,2] (CEPPs) were converted to the Kleinman-Bylander form[3] and tabulated on a radial grid as required for the CASTEP code[4]. Projection orbitals were obtained from atomic calculations using the tabulated pseudopotentials. For O, the pseudopotential represents a He core, the local channel is $d$, and a projector was generated for both the $s$ and $p$ channels from ground-state atomic orbitals. For Ti, the pseudopotential represents a Ne core, and the local channel is $f$. Due to the semi-core nature of the Ti CEPP, five projectors were used, requiring some minor modifications to the CASTEP code. Two $s$ projectors, one $p$ projector, and one $d$ projector were taken from the ground-state pseudoatom orbitals, with an additional $p$ projector taken as the $4p$ orbital of the $3s^2 3p^6 4s 3d^2 4p$ excited state (the lowest energy state with an occupied $4p$ orbital).

For both Ti and O pseudopotential, projectors were generated using the PBEsol functional[5] and the numerical-grid atomic DFT code available as part of the ESPRESSO package[6]. With pseudopotentials replacing cores, each $TiO_2$ possesses 24 valence electrons.

Within QMC it is only possible to perform calculations with one Bloch vector, $\mathbf{k}_s$, where "s" stands for "supercell". A single $\mathbf{k}_s$ associated with a supercell of many primitive unit cells is generally equivalent to an offset Monkhorst-Pack grid for the primitive unit cell[7,8]. In light of this equivalence, an optimum supercell geometry and $\mathbf{k}_s$ was generated, with the associated primitive cell and $\mathbf{k}$-point grid used explicitly for the DFT calculations.

We chose simulation cells that maximize the distance between periodic images[9], which mitigates finite size errors[10,11].

The $\mathbf{k}_s$ vectors were chosen such that the wave functions were real, which improves the computational efficiency but reduces the number of candidate $\mathbf{k}_s$ values to eight. For each candidate $\mathbf{k}_s$ the DFT total energy was calculated and the $\mathbf{k}_s$ that gave an energy closest to that of the dense $\mathbf{k}$-point limit was selected. For the optimum supercells and selected $\mathbf{k}_s$, the largest deviation from the dense $\mathbf{k}$-point limit is $-0.0064$ eV/[$TiO_2$] (the finite-size corrections described below correct this error).

For the systems considered, the dense $\mathbf{k}$-point limit was approximated as the energy resulting from a Monkhorst-Pack set with an estimated convergence error of 0.0003 eV/[$TiO_2$], or better.

The basis sets used correspond to an energy cut-off of 160 Ry (2176.9108 eV), providing DFT total energies that differ from the large basis set limit by approximately 0.42 eV/[$TiO_2$] for all four structures, and energy differences that deviate from the large basis set limit by $< 0.0036$ eV/[$TiO_2$].

## II. DETAILS OF THE DMC CALCULATIONS

Plane wave orbitals resulting from the DFT calculations were transformed into a 'blip' polynomial representation[12] to improve the computational efficiency of the DMC calculations. Note that we used the same Jastrow factor[13,14] parameters for each $\mathbf{k}_s$ point studied.

DMC calculations were performed using the optimum 768 electron supercell and trial wave function for each structure, and a time step of $\tau = 0.004$ a.u. To validate this choice of time-step the associated error was quantified by performing test DMC calculations for a smaller 192-electron optimum supercell at time steps of $\tau = 0.001$, 0.0025, and 0.004 a.u. and extrapolating the results to zero time step[15]. The data and extrapolations arising from such calculations are shown in Fig. 1, demonstrating that time-step errors in the energy differences between polymorphs are $< 0.002$ eV/[$TiO_2$], which is negligible when compared with the target accuracy of 0.01 eV/[$TiO_2$].

### A. Finite-size errors

To reduce systematic errors for extended systems we include accurate corrections to errors arising from the finite supercell sizes. We used the method of Kwee *et*

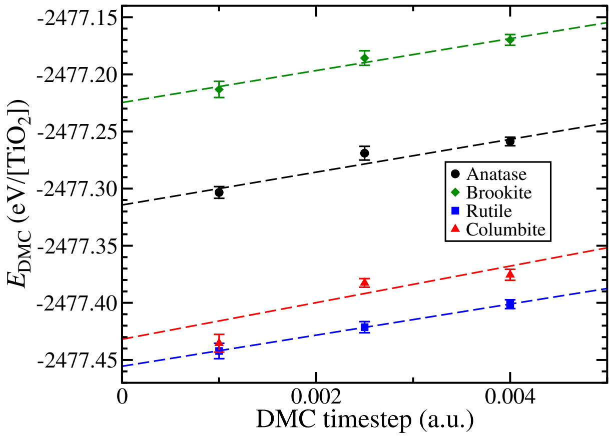


FIG. 1. DMC energies of the four polymorphs of $TiO_2$ as a function of DMC time-step for the 192 electron unit cell.

*al.*[16] that involves DFT calculations using an alternative LDA functional (the "KZK" functional) constructed from DMC data for homogeneous electron gases in supercells of different sizes. The KZK finite size corrections were corrected for finite basis set errors using results from PBEsol-DFT calculations with plane-wave cutoff energies of 150, 155, and 160 Ry.

The finite-size corrected DMC energy, $E_{\rm DMC}(\infty)$, is obtained from the results of DMC finite supercell calculations, $E_{\rm DMC}(N)$, and using

$$E_{\rm DMC}(\infty) = E_{\rm DMC}(N) + [E_{\rm LDA}(\infty) - E_{\rm LDA}(N)] - [E_{\rm LDA}(N) - E_{\rm KZK}(N)] \quad , (1)$$

where $E_{\rm LDA}(N)$ is the LDA total energy arising from the sparse **k**-point grid corresponding to an optimum supercell, and $E_{\rm KZK}(N)$ is the KZK total energy arising from the sparse **k**-point grid corresponding to the optimum supercell. For both cases the size of the optimum supercell is indexed by the number of electrons within it, $N$. The LDA result for the continuous **k**-point grid, $E_{\rm LDA}(\infty)$, was approximated using a dense Monkhorst-Pack grid with a **k**-point spacing of 0.035 Å$^{-1}$. The resulting total energies differ from those obtained for a grid spacing of 0.060 Å$^{-1}$ by less than 0.0003 eV/[$TiO_2$], so may be considered as well converged.

The first bracketed term in Eq. (1) is a one-body component of the correction due to the finite supercell in the underlying DFT calculation, whereas the second bracketed term is a two-body correction due to the non-physical correlation between electrons and their periodic images. We estimate the accuracy of both the one- and two-body terms when applying the KZK correction.

The two-body corrections for 32 $TiO_2$ units evaluated in Eq. (1) lie in the range 0.2526–0.2756 eV/[$TiO_2$] for the four structures considered. The error in the two-body term is straightforward to quantify. Both LDA and KZK results were generated for optimum supercells containing 16, 24, and 32 $TiO_2$ units, and the resulting correction was extrapolated accurately to an infinite supercell using $E_{\rm LDA}(N) - E_{\rm KZK}(N) = \epsilon_2 + a_2/N$, where $\epsilon_2$ and $a_2$ are fitting parameters (see Fig. 2). The errors in these corrections are estimated consistently across the four structures as $\epsilon_2 = -0.0031$ eV/[$TiO_2$].

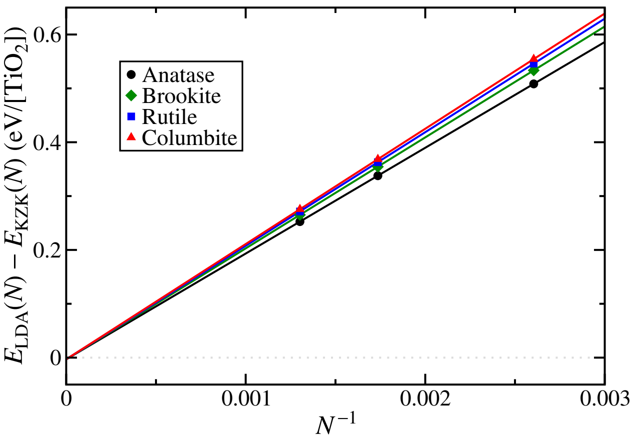


FIG. 2. Convergence of two-body finite size corrections with the number of electrons in the supercell, $N$. Calculated two-body corrections deviate from the fitted linear behavior by $1.1 \times 10^{-5}$ eV/[$TiO_2$], or less. Estimated errors ($\epsilon_2$) are provided by the two-body correction linearly extrapolated to the $N \to \infty$ limit for each structure.

For the one-body term such a linear extrapolation is not applicable (see Fig. 3). The error was estimated as the largest absolute difference between one-body corrections evaluated using LDA functionals and GGA functionals. The maximum was taken over the all supercells, all polymorphs, all available GGA functionals (PBE[17], PBEsol[5], PW91[18], rPBE[19], and WC[20]), and occurred for brookite with 16 $TiO_2$ units and the rPBE functional. This provides an estimated one-body error of 0.0017 eV/[$TiO_2$].

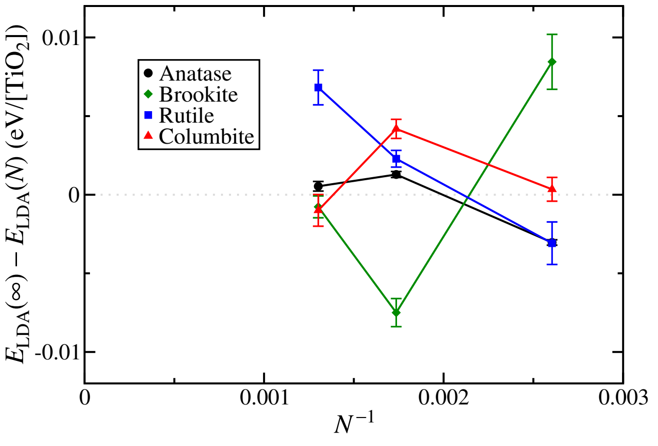


FIG. 3. One-body finite size correction evaluated for each structure and supercell (containing $N$ electrons). Error bars for each one-body finite size correction are evaluated as described in the text.

Calculated finite size corrections perform marginally

better than previous applications of the KZK method, with the maximum error in the finite size correction being 0.0037 eV/atom for a 74-atom $TiO_2$ supercell, to be compared a bulk Si finite-size-correction error of 0.007 eV/atom for a 54-atom supercell[21].

## III. DETAILS OF THE VIBRATIONAL CORRECTIONS

The vibrational calculations have been performed with our own code using DFT-PBEsol[5] energies obtained from the CASTEP[4] code.

We have performed harmonic vibrational calculations on all four structures considered, using the finite-displacement method together with the non-diagonal supercells approach[22]. Nondiagonal supercells allow us to access large vibrational Brillouin zone wavevector grids with moderate supercell sizes without any loss of accuracy. We have used $4\times4\times4$ grids for the rutile, anatase, and columbite structures, and a $2\times2\times2$ grid for the brookite structure. Symmetry-inequivalent positive and negative finite displacements of 0.005 Å have been used to construct the matrix of force constants, which has been Fourier-transformed to obtain the corresponding dynamical matrices, which in turn are diagonalized to calculate the vibrational harmonic frequencies and eigenvectors. Using this approach, imaginary-frequency modes are found to be present in the rutile structure, indicating lattice instability. For example, there are two such unstable modes at the Brillouin zone center Γ, and we have checked that these modes are present for a range of functionals, demonstrating that they have a physical origin and are not artifacts of the approximations employed (see Fig. 4).

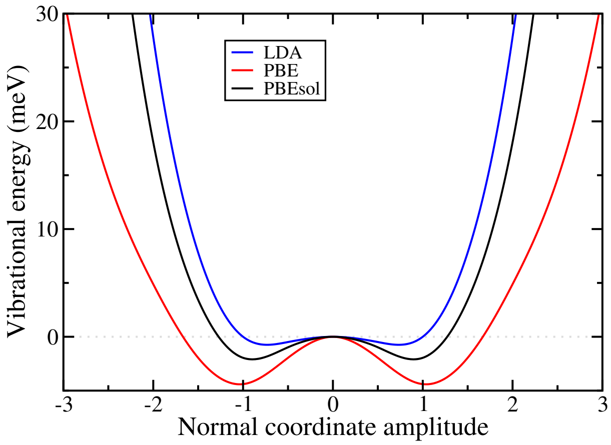


FIG. 4. A slice through the Born-Oppenheimer energy surface for an imaginary-frequency mode present in the rutile structure at the Γ point of the vibrational Brillouin zone. The three curves correspond to the LDA, PBE, and PBEsol functionals. The normal coordinate is measured in units of $1/\sqrt{2|\omega|}$, where $\omega$ is the imaginary harmonic frequency of the mode.

The presence of dynamical instabilities in the rutile structure means that it is necessary to go beyond the harmonic approximation to obtain reliable results for the vibrational contribution to the energy.

We have performed anharmonic vibrational calculation for all structures considered using the method described in Ref. 23. The Born-Oppenheimer energy surface is mapped along the harmonic normal modes of vibration out to large amplitudes with 16 sampling points along each direction. All modes of the harmonic grids considered above are mapped in this way, and the results are used to construct an anharmonic approximation to the Born-Oppenheimer energy surface. The use of nondiagonal supercells has proved crucial for obtaining results that are converged with respect to the simulation cell size. The resulting vibrational anharmonic Hamiltonian is solved by employing a mean-field ansatz for the vibrational wave function, and the anharmonic vibrational eigenvalues are then used to calculate the anharmonic vibrational zero-point energy and Helmholtz free energy. The anharmonic calculations show that all of the structures are dynamically stable, even at zero temperature.

### A. Quantifying anharmonicity

While the Born-Oppenheimer energy surface of rutile exhibits evident anharmonicity, it is useful to quantify the degree to which this anharmonicity affects the Helmholtz free energies which make up our main results. Typically, the effect of anharmonicity can be thought of as an "anharmonic correction" which is solely determined by the difference between harmonic and anharmonic vibrational eigenvalues. However, when dynamical instabilities are encountered in harmonic vibrational calculations it is common practice to simply ignore the contribution from unstable modes in harmonic estimates of vibrational expectation values. This approach introduces a methodological bias in the harmonic results which we analyze separately.

It is not possible to evaluate the methodological bias incurred by ignoring unstable modes in harmonic calculations, since the missing harmonic contributions to the free energy are not well defined, and we quantify this bias by evaluating its anharmonic counterpart instead. In Fig. 5 we plot the difference between the anharmonic free energy ignoring modes which are unstable at the harmonic level and the anharmonic free energy including contributions from all vibrational modes. We only consider the rutile and columbite polymorphs, since anatase and brookite $TiO_2$ do not exhibit unstable modes in our harmonic calculations. The methodological bias for the columbite polymorph is small over the temperature range considered, while that for rutile $TiO_2$ grows rapidly in magnitude with temperature, exceeding our target accuracy of 0.01 eV/[$TiO_2$] slightly above 300 K.

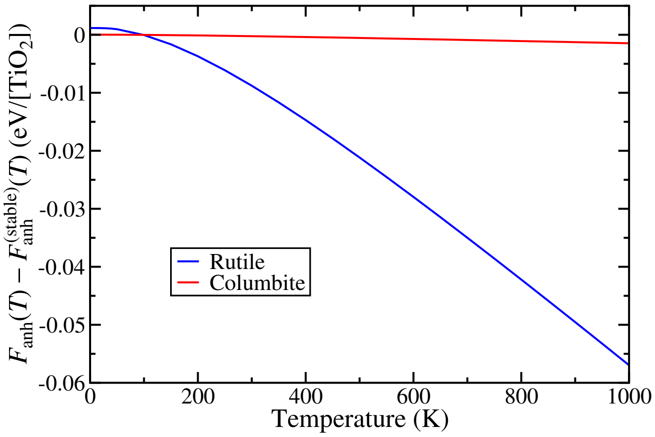


FIG. 5. Difference between the anharmonic contribution to the free energy from modes which are stable at the harmonic level ($F_{anh}^{(stable)}$) and the total anharmonic free energy ($F_{anh}$) of rutile and columbite $TiO_2$ as a function of temperature. This difference is an approximation to the methodological bias incurred by ignoring unstable modes in the evaluation of the free energy within the harmonic approximation.

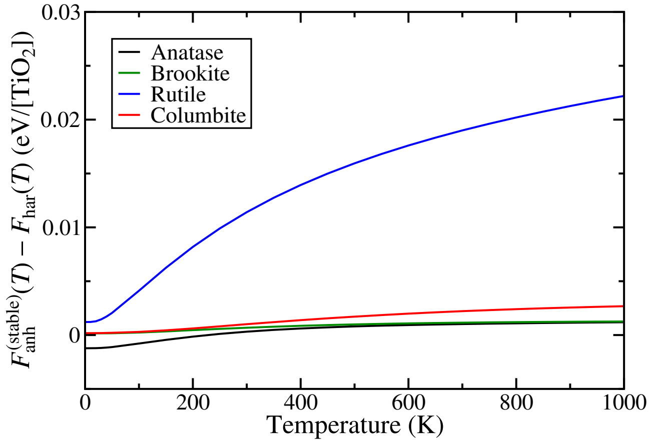


FIG. 6. Difference between the harmonic ($F_{har}$) and anharmonic ($F_{anh}^{(stable)}$) contribution to the free energy from modes which are stable at the harmonic level as a function of temperature. This difference is a measure of the degree of anharmonicity of the modes which can be described by the harmonic approximation.

We quantify the distinct "anharmonic correction" due to differences in harmonic and anharmonic vibrational eigenvalues by plotting the difference between the harmonic and anharmonic contributions to the free energy from modes which are stable at the harmonic level, see Fig. 6. This measure of anharmonicity is small for the anatase, brookite, and columbite polymorphs, but for rutile $TiO_2$ it exceeds our target accuracy of 0.01 eV/[$TiO_2$] for temperatures above 300 K.

We note that the biases plotted in Figs. 5 and 6 add up to the difference between the estimate of the free energy that would typically be obtained within the harmonic approximation and the anharmonic free energy. Since the errors for rutile $TiO_2$ are of opposite sign over much of the temperature range considered, using the harmonic approximation in the manner described would give reasonable estimates of the Helmholtz free energies for temperatures of up to 600 K. However this cancellation of errors is fortuitous, and the present analysis demonstrates the large degree of anharmonicity exhibited by rutile $TiO_2$, which confirms the importance of including anharmonicity in the study of this polymorph.

### B. Thermal expansion

In the paper we analyze the effect of neglecting thermal expansion in our calculations by calculating the difference between the Helmholtz free energies of anatase and rutile $TiO_2$ at both the fixed-volume geometries and using variable-volume experimental unit cell geometries[24] within the harmonic approximation. We estimate that the error incurred by neglecting thermal expansion in our calculations is less than 0.003 eV/[$TiO_2$] over the temperature range 300–575 K.

We note that for rutile $TiO_2$ above 575 K the harmonic estimation of the thermal expansion error becomes inaccurate because the variable-volume system experiences a rapid increase in the proportion of unstable harmonic modes that need to be excluded from the evaluation of the Helmholtz free energy. This renders the underlying harmonic approximation unreliable, and as a consequence we are unable to quantify the error incurred by neglecting thermal expansion at temperatures above 575 K.


[1] J. R. Trail and R. J. Needs, J. Chem. Phys. **139**, 014101 (2013).
[2] J. R. Trail and R. J. Needs, J. Chem. Phys. **142**, 064110 (2015).
[3] X. Gonze, R. Stumpf, and M. Scheffler, Phys. Rev. B **44**, 8503 (1991).
[4] S. J. Clark, M. D. Segall, C. J. Pickard, P. J. Hasnip, M. I. J. Probert, K. Refson, and M. C. Payne, Z. Kristallogr. **220**, 567 (2005)
[5] J. P. Perdew, A. Ruzsinszky, G. I. Csonka, O. A. Vydrov, G. E. Scuseria, L. A. Constantin, X. Zhou, and K. Burke, Phys. Rev. Lett. **100**, 136406 (2008); Erratum Phys. Rev. Lett. **102**, 039902(E) (2009).
[6] P. Giannozzi et al., J. Phys.: Condens. Matter **21** 395502 (2009); `http://www.quantum-espresso.org`.
[7] G. Rajagopal, R. J. Needs, S. Kenny, W. M. C. Foulkes, and A. James, Phys. Rev. Lett. **73**, 1959 (1994).
[8] G. Rajagopal, R. J. Needs, A. James, S. D. Kenny, and W.

M. C. Foulkes, Phys. Rev. B **51**, 10591 (1995).
[9] N. D. Drummond, B. Monserrat, J. H. Lloyd-Williams, P. López Ríos, C. J. Pickard, and R. J. Needs, Nat. Commun. **6**, 7794 (2015)
[10] N. D. Drummond, R. J. Needs, A. Sorouri, and W. M. C. Foulkes, Phys. Rev. B **78**, 125106 (2008); Erratum Phys. Rev. B **90**, 159901(E) (2014).
[11] P. R. C. Kent, R. Q. Hood, A. J. Williamson, R. J. Needs, W. M. C. Foulkes, and G. Rajagopal, Phys. Rev. B **59**, 1917 (1999).
[12] D. Alfe and M. J. Gillan, Phys. Rev. B **70**, 161101 (2004).
[13] N. D. Drummond, M. D. Towler, and R. J. Needs, Phys. Rev. B **70**, 235119 (2004).
[14] P. López Ríos, P. Seth, N. D. Drummond, and R. J. Needs, Phys. Rev. E **86**, 036703 (2012).
[15] R. M. Lee, G. J. Conduit, N. Nemec, P. López Ríos, and N. D. Drummond, Phys. Rev. E **83**, 066706 (2011); Erratum Phys. Rev. E **85**, 029908(E) (2012).
[16] H. Kwee, S. Zhang, and H. Krakauer, Phys. Rev. Lett. **100**, 126404 (2008).
[17] J. P. Perdew, K. Burke and M. Ernzerhof, Phys. Rev. Lett. **77**, 3865 (1996).
[18] J. P. Perdew, J. A. Chevary, S. H. Vosko, K. A. Jackson, M. R. Pederson, D. J. Singh and C. Fiolhais, Phys. Rev. B **46**, 6671 (1992).
[19] B. Hammer, L. B. Hansen and J. K. Norskov, Phys. Rev. B **59**, 7413 (1999).
[20] Z. Wu and R. E. Cohen, Phys. Rev. B **73**, 235116 (2006).
[21] R. Maezono, N. D. Drummond, A. Ma, and R. J. Needs, Phys. Rev. B **82**, 184108 (2010).
[22] J. H. Lloyd-Williams and B. Monserrat, Phys. Rev. B **92**, 184301 (2015).
[23] B. Monserrat, N. D. Drummond, and R. J. Needs, Phys. Rev. B **87**, 144302 (2013).
[24] D. R. Hummer, P. J. Heaney, and J. E. Post, Powder Diffr. **22**, 10095 (2007).
